# Supplementary material for: Worst-Case Detection Performance for Distributed SIMO Physical Layer Authentication
Source: arXiv:2005.06793 source file (2020-10-12)
Supplement: Supplementary file 1 [file TCOM-2020-Additional-Notes.pdf]

# Worst-Case Detection Performance for Distributed SIMO Physical Layer Authentication

Notes on the Resubmission

Henrik Forssell

Ragnar Thobaben

October 11, 2020

## Abstract

This document contains additional notes on our submission "Worst-Case Detection Performance for Distributed SIMO Physical Layer Authentication". Since the previous version of the paper<sup>1</sup> was rejected for publication in the *IEEE Transactions on Wireless Communications* earlier this year, we have carefully revised the manuscript based on the received criticism. In this document, we first summarize the major modifications made to the first submission, and then, provide all comments from the previous review along with our responses.

## Summary of Modifications

First, we note that all modifications to the previous submission are highlighted in blue in the revised manuscript. The major modifications are:

- We have changed the title of the paper to "Worst-Case Detection Performance for Distributed SIMO Physical Layer Authentication". The purpose is to highlight our focus on *worst-case* detection performance guarantees that differentiates our work from most previous works on physical layer authentication (PLA). Such guarantees for optimized attack strategies (i.e., for optimal transmit power and position of the attacker) have not been provided by previous works. We note therefore that the main contribution of this paper is the provided method to derive the missed detection probability for a worst-case attacker, and the considered PLA scheme provides a relevant context that mimics properties of distributed antenna array technologies in 4G and 5G RANs.

---

<sup>1</sup>The previously submitted version was titled "Distributed SIMO Physical Layer Authentication: Performance Bounds Under Optimal Attacker Strategies".

- The introduction in Section I has been revised to better highlight the motivation, the relevance, and contributions of this work. Several reviewers requested better references to related work and, with this in mind, we have added a separate Section I.B devoted to previous works. In Section I.B, we have extended the discussion of the references [1, 2, 3] that previously have considered attack strategies against PLA, in order to clarify the differences and similarities to our approach. Moreover, Section I.B now covers related works that employ the same GLRT hypothesis test, PLA based on angle-of-arrival or line-of-sight beam-forming, and machine-learning approaches.
- Two paragraphs have been added in Section II.B that clarify the relation between the authentication scheme and the assumed channel model, and to discuss system-level impacts from the distributed antenna architecture.
- Section II.C and Section II.E have been revised to more clearly explain the problem formulation and its relation to the choice of authentication threshold.
- We have removed a subsection of Section III that previously discussed generalization of the results to imperfect CSI. This was necessary to make space for the required changes and to expand the discussions in other parts of the paper. Instead, the imperfect CSI extension is mentioned in a footnote.
- We have removed two result plots in Section V that served as additional validation of the saddle-point approximation accuracy. This was necessary to make space for the required changes and to expand the discussions in other parts of the paper.
- The discussion of the numerical results in Section V.E has been extended, specifically to discuss how the results relate to previous PLA schemes.

In the following sections, we provide the entire feedback received from the editor and reviewers regarding the first submission of the paper. We address each comment and point to the corresponding modifications we have made for the resubmission.

## Response to Editor

- 0.1. *"Although the reviewers found the topic interesting, they raised some major concerns of the manuscript. Specifically, there are unjustified assumptions about the attacker's capability in the model; for example, the derived attacking strategies at Eve are based on the knowledge of Alice's channel statistics. How to compute the PFA and determine the threshold in the proposed approach are not available, casting doubt on its practicality. All reviewers pointed out that there is no comparison of the proposed approach with existing PLA schemes to demonstrate the advantage and difference of the proposed scheme over the existing methods. These undermine the novelty and contribution of this work."*

**Response:** The criticism received from the Editor is based on the comments provided by the reviewers. Our respective responses to these issues will be provided in detail in the following sections.

## Response to Reviewer 1

- 1.1. *"This paper an array-based physical-layer authentication scheme based on the single-input multiple-output channel states to resist the power manipulation attacks and the spatial position attacks. This scheme builds a hypothesis test to authenticate the messages and derives the worst-case detection bounds in terms of the false alarm rate and the miss detection rate. Numerical results show that the proposed scheme reduces the false alarm rate and the miss detection rate. However, this paper does not provide experiments to verify the effectiveness of the proposed scheme."*

**Response:** The paper reports results from experiments in terms of system simulations that are based on the statistical models that were used throughout the paper, in order to evaluate and verify the derived performance bounds on the missed detection probability. Specifically, the simulations are based on independent channel realizations that are drawn from the considered fading distributions with location-dependent parameters of the fading distribution based on the two-dimensional deployment scenario shown in Fig. 3. This is a well-establish approach to validate the correctness of performance bounds in a system context. We agree that an experimental validation based on a testbed radio platform would be interesting. Unfortunately, in this work we do not have the resources for a real-world implementation with multiple antenna arrays, and we currently do not have access to channel measurements that fit the considered scenario. Such evaluations are left for future work.

In the revised manuscript we have improved and clarified the description of the numerical evaluation scenario in Section V so as to avoid confusion around what experiments we have conducted.

- 1.2. *"What are the advantages of the proposed scheme compared with the existing feature-based physical-layer authentication schemes?"*

**Response:** We first want to emphasize that the contribution of this paper is not limited by the particular advantages of the distributed physical layer authentication (PLA) scheme studied in this paper. First and foremost, we provide worst-case analysis for the PLA scheme in terms of upper bounds on the missed detection probability under the power manipulation attack and the optimal position attack. The results obtained for the optimal power manipulation attack can be applied to a wide variety of other PLA schemes as well. Since the PLA scheme we consider is based on a generalized likelihood-ratio test (GLRT) similar to previously proposed PLA schemes [4, 5, 1], our results can be used to evaluated the worst-case performance of these schemes and their extension to a distributed detection framework as well.

The advantage of the distributed antenna approach, compared to the co-located antenna case, lies in its resilience to the optimal position attack. The attack strategy against a single multiple-antenna radio-head is more straightforward: Choose the same angle-of-arrival (AoA) as the legitimate device and adapt the transmit power to match the received power from the legitimate transmitter. With multiple distributed radio-heads, however, the optimal position is less trivial and the optimal success rate an attacker can achieve is reduced. The tools we develop in this paper allow us to quantify this effect, a problem that has not been solved before.

- 1.3. *"Why does each link have a light-of-sight component to each RRH? Please provide references to verify this assumption."*

**Response:**

In the paper, we make two assumptions regarding the channel distribution: (i) that it is non-zero mean (i.e., Rice fading) and (ii) that its mean vector follows the phased-array model in Eq. (1).

The central prerequisite for the PLA scheme is the first assumption (i), which from a physical perspective is relevant when there are few dominating (line-of-sight (LoS) or reflective) paths between transmitter and receiver (e.g., between sensor and access-points in a large open factory hall or between car and road-side access-points). Similar Rice fading models have been assumed in previous PLA works [6, 7] and in our previous works on multiple-antenna PLA [8, 9]. To briefly address generalizations to non-LoS channels, we note that the non-zero mean distribution in (i) also could represent the predictive distribution of a channel predictor (e.g., a Kalman filter).

The second assumption (ii) results in the particular phased-array form of the channel mean, which is dependent on a single LoS or reflective path with a particular distance and AoA. This model could be generalized to include multiple paths with individual lengths and AoAs; however, this was considered outside the scope of this work. The phased-array response model has previously been employed within physical layer security in [10]. Moreover, note that LoS channels is a common assumption within physical layer security e.g., exploited for jamming resilience [11] and protection against eavesdroppers and active attacks [10, 12]. There are as well experimental measurements that justify LoS assumption in indoor communication environments [13].

In the revised manuscript, the discussion of these assumptions has been extended in the added Section I.B and the closing paragraph in Section II.A regarding the channel model.

- 1.4. *"What is the meaning of  $CSI(m)$  in Section II-B?"*

**Response:** We agree that this notation was somewhat confusing and have removed it in the revised version of the paper.

- 1.5. *"What is the channel model of this scheme? Does this scheme depend on a specific channel model?"*

**Response:** The channel model assumed in this paper is Rice fading, narrowband, single-input multiple-output (SIMO) and it is defined in mathematical detail in Section II.A of the paper. However, the analysis of the power manipulation attack applies more generally to any feature-based PLA scheme based on GLRT tests. For details on the relationship between the channel assumptions and the PLA scheme, see also the response to Comment 1.3.

- 1.6. *"Provide experimental results based on realistic data to verify the effectiveness of the proposed scheme."*

**Response:**

The results provided in this paper is entirely based on numerical evaluations of the theoretical bounds and Monte Carlo simulations. Comparison to results based on real-world measurements was considered outside the scope of this work since we did not have the resources required to perform measurements in the considered system setups. The relevance of the models in relation to real-world systems is however discussed and this discussion has been expanded in the revised version of the paper (e.g., in the added parts of Section I.B and Section V.E).

- 1.7. *"How does the authentication latency of this scheme change with the total number of antennas in Section V?"*

**Response:**

Firstly, this paper does not quantify the latency impacts of the distributed PLA scheme. However, we do discuss system-level impacts and this discussion has been expanded in Section II.B of the revised manuscript. As we show in Section II.B, the PLA scheme only requires communication of one real-valued sample per authenticated message on each link from a RRH to Bob, an added overhead that can be argued to have little impact on the latency. In addition to this, false alarms will also influence the latency, something we previously have studied for co-located antennas in [8] and for distributed antennas in [9].

- 1.8. *"Provide simulation results to compare the authentication performance with existing PLA schemes."*

**Response:**

Our results allow us to compare the distributed PLA approach to the single-RRH case and demonstrate that the former is superior with respect to worst-case missed detection performance. Beyond this it is hard to make a meaningful numerical comparison

to other schemes (e.g., based on other feature choices like frequency or impulse responses) since the performance often is highly dependent on channel parameters like, e.g., frequency selectivity, bandwidth, and signal-to-noise ratio. Assuming a fair parameterization and scaling of other features (e.g., number of independent resolvable channel taps of the impulse response matches the number of antennas per array; same SNR), we expect however that the performance of GLRT based schemes that employ other features will coincide with the single-RRH case.

At this point, we note that the considered system model could be extended to a multi-carrier system (i.e., stacking the feature-vector corresponding to each sub-carrier for an OFDM channel), which would introduce an additional feature dimension and potentially improve detection performance. The performance improvements would depend on the correlation across sub-carriers and antennas. We have included a discussion on the relation of our results to multi-carrier schemes in Section V.E.

- 1.9. *"The references lack some important information such as the published year, volume, and issue. Please double-check."*

**Response:** We have completed all references with missing information in the revised version of the manuscript.

## Response to Reviewer 2

- 2.1. *"This paper considers two attacking strategies in Physical Layer Authentication (PLA). The topic is interesting but there are many serious concerns and unreasonable assumptions."*

**Response:** The issues raised by Reviewer 2 are replied to in the following responses.

- 2.2. *"Lack of comparison with current state-of-the-art methods. There are many PLA schemes proposed recently. The authors should provide a comprehensive comparison of the existing PLA scheme with the proposed approach in the experimental results."*

**Response:** We have significantly extended the references to other PLA schemes in Section I.B dedicated to related work. We have also improved the discussion of the numerical results in relation to previous schemes in Section V.E. Again, we want to emphasize that the main contribution is not the considered PLA scheme, but rather the methods for deriving worst-case detection performance under any attacker. Please see also response to Comment 1.2.

- 2.3. *"The authors did not explicitly provide the closed-form expressions of the PFA and the optimal threshold. Then, the proposed approach cannot be directly applied to practi-*

*cal situations. For example, an inappropriate threshold can cause various detection errors.”*

**Response:** This is a misunderstanding since the probability of false alarm was provided in closed form in Section II.C of the original manuscript.

Regarding the threshold choice, this design can fundamentally be viewed in different ways. For example, (i) the system designer determines a tolerable false-alarm rate (e.g., in order to satisfy latency constraints), computes the corresponding threshold, and obtains the worst-case missed detection probability as a security guarantee; (ii) the designer picks a given highest tolerable missed detection probability, computes the corresponding threshold, and obtains the associated false-alarm probability. (iii) the designer is given security and quality of service requirements in terms of missed detection and false alarm probability, and dimensions the system (e.g., number of RRHs and number of antennas per RRH) and optimizes the decision threshold to meet the requirements. Performing this in a practical setting essentially requires knowledge of the legitimate channel distribution, which is already necessary for the PLA scheme, and the geometry of the deployment area. We agree that an inappropriate threshold can cause detection errors, but our results allow us to quantify and bound the probability of such errors.

We have improved the description of the threshold design, explicitly stated the threshold for a given false-alarm probability in Eq. (5) in Section I.C, and updated the problem description in Section II-E to reflect the discussion above.

- 2.4. *”The authors assume that Eve can obtain Alice’s information when she launches an attack, e.g.,  $\mu_A$  and  $\Sigma_A$ . The authors should justify this assumption. In the papers that focus on attacking strategies, the authors cannot unreasonably enhance the attacker’s capability, which is meaningless.”*

**Response:** The focus of this paper is on worst-case performance guarantees. Therefore, we believe that it is justified to assume the worst-case attacker so as to properly characterize the worst-case detection performance. Such notions of a worst-case attacker are not uncommon within the area of physical layer security. In our work, we have assumed an attacker that perfectly knows the statistics of the legitimate channel. Practically speaking, the attacker could use knowledge of the positions, environment, and ray-tracing tools to infer this distribution or, alternatively, the features could easily leak to the attacker if the PLA feature bank is public knowledge. Moreover, while introducing channel uncertainty at Eve is an interesting problem, it would only degrade the attacker’s success probability, i.e., the results in this paper still apply as worst-case bounds.

In the revised manuscript, we have modified the beginning of Section III.A to make this assumption and our justification more clear.

- 2.5. *"This paper does not provide any new insight into the PLA. For example, the channel-based PLA scheme distinguishes Alice and Eve by comparing the channel response. Apparently, if Eve is closer to Alice, Eve can obtain more attacking gain. Without the complicated derivations provided in this paper, we can easily obtain the above conclusion as well."*

**Response:** The analytical results we provide in this paper allow us to formally guarantee the detection performance of the PLA scheme. Moreover, they are useful for studying how the detection performance behaves with various parameters such as position, LoS strength, fading correlation, etc. Of course many of the obtained results are consistent with intuition; however, they also allow us to provide new insights and quantify the results in *exact probabilities*. Examples of such insights are: (i) the benefits of the distributed approach ( $N_{\text{RRH}} > 1$ ) compared to a co-located scenario ( $N_{\text{RRH}} = 1$ ), (ii) that no additional performance gains were obtained by distributing antennas to more than two locations, and (iii) the ordering of side-lobe intersections in the optimization of the attack position.

- 2.6. *"Some formulas did not provide any necessary explanations.*

- (a) *For example, Eq. (4), Is it the best choice for a test statistic?*
- (b) *How does the factor  $K_{\text{Rice}}$  affect performance?"*

**Response:**

- (a) The decision statistic in Eq. (4) is based on the generalized likelihood-ratio test (GLRT) used in many related works on feature-based PLA [4, 5, 1] (see [14, Chapter 4.2.7] for a textbook definition). It is the optimal test for Gaussian features when the receiver does not know the attacker's distribution.
- (b) The effect of the Rice factor  $K_{\text{Rice}}$  can be seen in Figure 4, 5, and 6(b). A higher Rice factor implies stronger line-of-sight path to the receiver and weaker random component due to scattering. This results in increasingly deterministic channels which improves detection performance since the channels become easier for Bob to distinguish between.

- 2.7. *"In the experimental results, the authors only provide many results but without any explanations, which is difficult to follow."*

**Response:** In the revised version of the paper, we have removed two plots that previously depicted the missed detection probability for varying attack position and number of antennas. The purpose is to make Section V less dense, improve the readability, and to allow room for the extended discussion in Section V.E. The removed plots are included in Figure 1 of this document and they show that the saddle-point approximation is accurate for both varying attack position (along the  $x$ -axis) and total number of antennas  $N_{\text{RRH}}N_{\text{Rx}}$ .

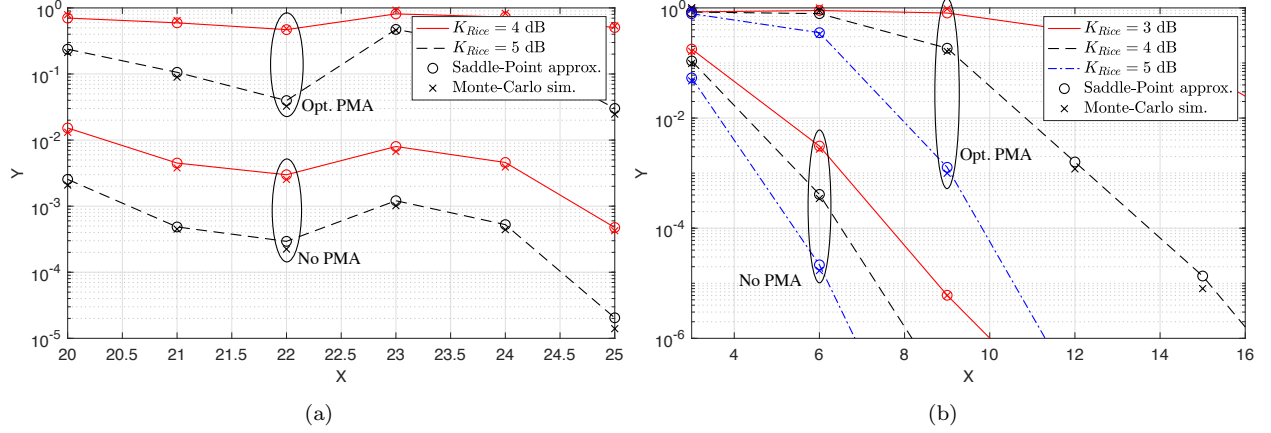

Figure 1: Saddle-point approximation of  $p_{\text{MD}}^{(\text{Opt. PMA})}$  compared to Monte-Carlo simulations for a  $N_{\text{RRH}} = 3$  RRH deployment for: (a) small variations in Eve's position and (b) varying correlation coefficient  $\rho$ .

2.8. *"Can the proposed approach only be applied to a distributed system? I strongly suggest the authors first investigate the performance of the proposed approach in an end-to-end system and then extend it to a distributed system."*

**Response:** This work specifically focuses on PLA in the distributed RRH setting. However, parts of the results also apply to the non-distributed setting (i.e., by letting  $N_{\text{RRH}} = 1$ ). For example, Theorem 1 gives the worst-case missed detection probability in closed form for  $N_{\text{RRH}} = 1$  which gives us the performance bound for the single-RRH system.

2.9. *"Alice should be put into Fig. 1."*

**Response:** In the first submission, Fig.1 consisted of multiple legitimate transmitters. We agree with the reviewer that it is better to have a single device named Alice and have updated the figure accordingly.

2.10. *"There are many confusing statements and typos. For example:*

- (a) *In Line 48 of Page 2, there are 'such as' and 'for example' simultaneously.*
- (b) *In Line 39 of Page 11, there missed a comma before  $k = 2$ .*
- (c) *In Line 42 of Page 16,  $r_k$  should be  $r_j$ .*
- (d) *In Line 30 of Page 19, there are two 'find'."*

**Response:** We appreciate that the reviewer pointed out these typos and have corrected them in the second revision of the paper.

## Response to Reviewer 3

- 3.1. *"Authors propose and analyze different strategies for an attacker to cheat the receiver in physical layer authentication, considering multiple remote radio-heads (RRHs). In general, the studied topic is very timely and the ideas are interesting. In particular, it is proved that there is no performance improvement from distributing antennas on more than two RRHs."*

**Response:** This summarizes our contributions. We would like to further emphasize that our results allow us to give detection performance guarantees that hold regardless of the attackers power manipulation strategy and choice of position.

- 3.2. *"Literature review could be improved by including a subsection devoted to related work."*

**Response:** We have significantly extended the discussion around related works in Section I.B of the revised manuscript.

- 3.3. *"The model examined suffers from some limitation, for example the fact the channel variations over time are not considered. How this would impact on the results?"*

**Response:** In this paper, we assume Rice fading channels where realizations vary from time-slot to time-slot. However, we assume time-invariant statistics representing channels from stationary users. In the case of user mobility, as long as the exact or predicted position of Alice is known at Bob and the corresponding predictive distribution of the channel feature can be inferred by Bob (e.g., by using channel tracking with a Kalman filter), the studied PLA scheme could be used in the same way. Extending the results to include transmitter mobility was however considered outside the scope of this work. This is discussed in the paragraph on feature learning in Section II.B.

- 3.4. *"Threshold  $T$  should be defined right after equation (3)."*

**Response:** This has been added in the revised manuscript.

- 3.5. *"In Section IV it is stated that the attacker's position is optimized excluding positions that are in the "immediate neighborhood" of the legitimate device. Could this proximity be defined more appropriately?"*

**Response:** The allowed positions are defined in terms of the region of positions  $\mathcal{R}$  in Definition 6. This region can be arbitrarily defined but in the numerical results we define it as all positions at a distance of more than 5 m from Alice.

- 3.6. *"Fig. 5a exhibits a non-monotonic trend and seems to suggest that there are positions which lead to local minima for the missed detection probability. Can this effect be predicted analytically? I suggest to add some comment to clarify this aspect."*

**Response:** This is exactly the theoretical observation we make in Section IV (specifically the observations following Lemma 3). Moreover, we show that we can efficiently sample the local maxima of the missed detection probability in the numerical results of Section V.B (specifically Fig. 7(a)).

- 3.7. *"Author could compare their results with those obtained by other physical layer authentication methods in the literature, in order to highlight the novelty and the difference in terms of performance with respects to the bounds found in the paper."*

**Response:** Please see response to Comment 1.8.

## References

- [1] P. Baracca, N. Laurenti, and S. Tomasin, "Physical layer authentication over MIMO fading wiretap channels," *IEEE Transactions on Wireless Communications*, vol. 11, no. 7, pp. 2564–2573, July 2012.
- [2] M. K. Shukla, A. Trivedi, and O. J. Pandey, "Physical layer authentication for mobile terminals over MIMO fading wiretap channels," in *International Conference on Advances in Computing, Communications and Informatics*, Aug 2013, pp. 638–642.
- [3] L. Senigagliesi, M. Baldi, and E. Gambi, "Performance of statistical and machine learning techniques for physical layer authentication," *CoRR*, Jan 2020. [Online]. Available: <https://arxiv.org/abs/2001.06238>
- [4] L. Xiao, L. Greenstein, N. Mandayam, and W. Trappe, "Fingerprints in the ether: Using the physical layer for wireless authentication," in *IEEE International Conference on Communications*, June 2007, pp. 4646–4651.
- [5] —, "Using the physical layer for wireless authentication in time-variant channels," *IEEE Transactions on Wireless Communications*, vol. 7, no. 7, pp. 2571–2579, July 2008.
- [6] A. Abdelaziz, R. Burton, and C. E. Koksall, "Message authentication and secret key agreement in VANETs via angle of arrival," *CoRR*, Sep. 2016. [Online]. Available: <http://arxiv.org/abs/1609.03109>
- [7] A. Abdelaziz, C. E. Koksall, F. Barickman, R. Burton, J. Martin, and J. Weston, "Enhanced authentication based on angle of signal arrivals," *IEEE Transactions on Vehicular Technology*, vol. 68, no. 5, pp. 1–1, 2019.
- [8] H. Forssell, R. Thobaben, H. Al-Zubaidy, and J. Gross, "Physical layer authentication in mission-critical MTC networks: A security and delay performance analysis," *IEEE Journal on Selected Areas in Communications*, vol. 37, no. 4, pp. 795–808, April 2019.
- [9] H. Forssell, R. Thobaben, and J. Gross, "Performance analysis of distributed simo physical layer authentication," in *IEEE International Conference on Communications*, May 2019, pp. 1–6.
- [10] S. Yan and R. Malaney, "Line-of-sight based beamforming for security enhancements in wiretap channels," in *International Conference on IT Convergence and Security*, 2014, pp. 1–4.
- [11] W. Guo, H. Zhao, and Y. Tang, "Testbed for cooperative jamming cancellation in physical layer security," *IEEE Wireless Communications Letters*, vol. 9, no. 2, pp. 240–243, 2020.

- [12] D. Kapetanovic, G. Zheng, and F. Rusek, "Physical layer security for massive mimo: An overview on passive eavesdropping and active attacks," *IEEE Communications Magazine*, vol. 53, no. 6, pp. 21–27, 2015.
- [13] H. MacLeod, C. Loadman, and Z. Chen, "Experimental studies of the 2.4-GHz ISM wireless indoor channel," in *3rd Annual Communication Networks and Services Research Conference*, May 2005, pp. 63–68.
- [14] M. Basseville and I. V. Nikiforov, *Detection of Abrupt Changes: Theory and Application*. Prentice Hall, 1993.
